# Supplementary material for: Cyber risk and the cross-section of stock returns
Source: arXiv:2402.04775 source file (2024-03-05)
Supplement: Supplementary file 1 [file appendix.tex]

\begin{comment}
\clearpage
\begin{table}[h]
    \begin{adjustbox}{width=\textwidth,center}
    \begin{tabular}{lcccccc}
        %\hline
        \textbf{Method}  & \textbf{Vector Size} & \textbf{Window Size} & \textbf{Min Count} & \textbf{Sub-Sampling} & \textbf{Negative Sampling} & \textbf{Epoch} \\
        \cmidrule(lr){1-1} \cmidrule(lr){2-2} \cmidrule(lr){3-3} \cmidrule(lr){4-4} \cmidrule(lr){5-5} \cmidrule(lr){6-6} \cmidrule(lr){7-7} 
        %\hline
        DBOW  & 300 & 15 & 5 & $10^{-5}$ & 5 & 20 \\
        %\hline
    \end{tabular}
    \end{adjustbox}
    \caption{\textbf{Baseline doc2vec parameters}}\bigskip
    \footnotesize{This table reports the parameters of the baseline model of \cite{LauBaldwin2016}. \quotes{DBOW} stands for distributed bag-of-words.}    
    \label{tab:baseline_doc2vec_parameters}
\end{table}
\end{comment}



\begin{comment}
\clearpage
\begin{table}
\noindent\makebox[\textwidth]{%
    \begin{tabular}{cp{115mm}cc}
        \toprule
        \toprule
        Score & \multicolumn{1}{c}{Preprocessed paragraph} & Ticker & Tactic\\
        \hline
        \footnotesize 0.570 & \footnotesize possible cookies may become subject laws limiting prohibiting use term cookies refers information keyed specific server file pathway directory location stored user hard drive possibly without user knowledge used among things track demographic information target advertising & \footnotesize VSTY & \footnotesize Discovery\\
        \footnotesize 0.561 & \footnotesize cannot certain advances computer capabilities discoveries field cryptography developments result compromise breach algorithms use protect content transactions website proprietary information databases anyone able circumvent security measures misappropriate proprietary confidential customer company information cause interruptions operations & \footnotesize VSTY & \footnotesize Impact\\
        \footnotesize 0.558 & \footnotesize ordering delivery customers ready place order proceed shopping cart function directly checkout page orders placed online website via toll free telephone number customer service agents available take orders customers access internet uncomfortable placing order online & \footnotesize VSTY & \footnotesize Credential Access\\
        \footnotesize 0.557 & \footnotesize process allows identify catalogue embryonic stem cell clone dna sequence trapped gene select embryonic stem cell clones dna sequence generation knockout mice used gene trapping technology automated process create omnibank library frozen gene knockout embryonic stem cell clones identified dna sequence relational database & \footnotesize \footnotesize LXRX &  \footnotesize Persistence \\
        \footnotesize 0.556 & \footnotesize believe systematic biology driven approach technology platform makes possible provide substantial advantages alternative approaches drug target discovery particular believe comprehensive nature approach allows uncover potential drug targets within context mammalian physiology might missed narrowly focused efforts & \footnotesize LXRX & \footnotesize Discovery\\
        \footnotesize 0.554 & \footnotesize concerns security internet may reduce use website impede growth significant barrier confidential communications internet need security rely ssl encryption technology designed prevent customer credit card data transaction process current credit card practices merchant liable fraudulent credit card transactions case transactions process merchant obtain cardholder signature & \footnotesize VSTY & \footnotesize Credential Access\\
        \bottomrule
        \bottomrule
    \end{tabular}
}
\caption*{Table \ref*{tab:top_paragraphs_doc2vec_validation}: \textbf{Top scoring paragraphs from the doc2vec validation sample (continued)}}
\end{table}
\end{comment}




\begin{comment}
\clearpage
\begin{table}
\vspace{-2em}
\begin{adjustbox}{width=\textwidth,center}
    \noindent\makebox[\textwidth]{%
    \begin{tabular}{lc}
    \toprule
    \toprule
    \multicolumn{2}{c}{Dependent variable: Monthly Portfolio returns}\\
    \midrule
    %& (6)\\
    %\midrule
    Cyber risk &  \textbf{0.156}$^{*}$\\
    & [1.951]\\
    HML & \textbf{-0.116}\\
    & [-1.236] \\
    SMB & \textbf{0.200}\\
    & [0.951]\\
    RMW & \textbf{0.062}\\
    & [0.753]\\
    CMA & \textbf{-0.173}\\
    & [-0.925]\\
    \\
    Consumer Durables & \textbf{-0.013}\\
    & [-0.212]\\
    Manufacturing & \textbf{-0.094} \\
    & [-1.261]\\
    Energy & \textbf{0.059}\\
    & [0.645]\\
    Chemicals & \textbf{0.062}\\
    & [0.909]\\
    Telecommunications & \textbf{-0.162}$^{**}$\\
    & [-2.19]\\
    Retail & \textbf{0.139}\\
    & [1.272]\\
    Healthcare & \textbf{-0.003}\\
    & [-0.046]\\
    Finance & \textbf{-0.019}\\\
    & [-0.211]\\
    Constant & \textbf{1.329}$^{***}$\\
    & [4.081] \\
    \midrule
    $\overline{R2_{adj}}$ & 0.307\\
    MAPE & 0.636\\
    \hline
    \hline
    \end{tabular}}
    \end{adjustbox}
    \caption{\textbf{Fama-MacBeth regressions with industries}}\bigskip
    \footnotesize{This table reports the results of Fama-MacBeth regressions of 20 value-weighted portfolios sorted on their cyber risk. These portfolios are regressed on portfolio value-weighted betas with HML, SMB, MOM, RMW, CMA, and industry returns and on portfolio value-weighted cyber-risk every month. The betas are standardized before the second step-regressions and estimated with a two-year rolling window. HML and SMB refer to the book-to-market and size factors of \cite{FamaFrench1992}. CMA and RMW refer to the investment and operating profitability factors of \cite{FamaFrench2015}. The industries are from the Fama-French 12 industry classification. We drop the \quotes{Business Equipment}, \quotes{Consumer NonDurables}, and \quotes{Utilities} industries given the high colinearity with the other industries and factors (as measured by the Variance Inflation Factor). We also drop the \quotes{Other} category because it lacks interpretability. $\overline{R2_{adj}}$ is the average adjusted R-squared, and MAPE is the mean average pricing error. Newey-West t-statistics are reported in brackets. $^{*}$, $^{**}$, and $^{***}$ indicate significance at the 10\%, 5\% and 1\% levels, respectively. The period is from January 2009 to December 2022.}
    \label{tab:Fama_MacBeth_industries}
\end{table}


\clearpage
\begin{table}
\begin{adjustbox}{width=\textwidth,center}
    \noindent\makebox[\textwidth]{%
    \begin{tabular}{lc}
    \toprule
    \toprule
    \multicolumn{2}{c}{Monthly Portfolio returns}\\
    \midrule
    %& (7)\\
    %\midrule
    Market & \textbf{-0.033}\\
    & [-0.578]\\
    Cyber risk &  \textbf{0.176}$^{**}$\\
    & [2.103]\\
    HML & \textbf{-0.033}\\
    & [-0.293] \\
    SMB & \textbf{-0.042}\\
    & [-0.385]\\
    RMW & \textbf{-0.086}\\
    & [-1.150]\\
    CMA & \textbf{0.011}\\
    & [0.076]\\
    Constant & \textbf{1.362}$^{***}$\\
    & [5.015] \\
    \midrule
    $\overline{R2_{adj}}$ & 0.295\\
    MAPE & 1.243\\
    \hline
    \hline
    \end{tabular}
    }
    \end{adjustbox}
    \caption{\textbf{Fama-MacBeth regressions with additional test assets}}\bigskip
    \footnotesize{
    This table reports the results of Fama-MacBeth regressions of 20 value-weighted portfolios sorted on their cyber risk extended with an additional 11 industry portfolios. These portfolios are regressed on portfolio value-weighted betas with the market, HML, SMB, MOM, RMW, and CMA and on portfolio value-weighted cyber-risk every month. The betas are standardized before the second step-regressions and estimated with a two-year rolling window. HML and SMB refer to the book-to-market and size factors of \cite{FamaFrench1992}. CMA and RMW refer to the investment and operating profitability factors of \cite{FamaFrench2015}. The industries correspond to the Fama-French 12 industry classification with the \quotes{Other} category dropped because it lacks interpretability. $\overline{R2_{adj}}$ is the average adjusted R-squared, and MAPE is the mean average pricing error. Newey-West t-statistics are reported in brackets. $^{*}$, $^{**}$, and $^{***}$ indicate significance at the 10\%, 5\% and 1\% levels, respectively. The period is from January 2009 to December 2022.}
    \label{tab:Fama_MacBeth_extended}
\end{table}
\end{comment}
